# Supplementary material for: FLORA: Unsupervised Knowledge Graph Alignment by Fuzzy Logic
Source: arXiv:2510.20467 source file (2025-10-23)
Supplement: Supplementary file 1 [file appendix.tex]

\section{Statistics of Datasets}

Table~\ref{tab:statistic_ea} and Table~\ref{tab:statistic_kga} summarize the statistics of the datasets used in our experiments. Following AttrGNN~\cite{attrgnn}, we use the DBP15K version enriched with attribute values from the DBpedia dump (2016-10). 
We exclude OpenEA D–Y~\cite{openea} due to its name bias, as almost all aligned entities in DBpedia and YAGO share the same names~\cite{prase}. We also discard the SRPRS~\cite{guo2019learning} and DWY100K~\cite{bootea} datasets, as they achieve perfect results using simple name-based heuristics~\cite{2020experimental}.

\begin{table}
\centering
\caption{Statistics of Entity Alignment datasets. ZH denotes Chinese, JA denotes Japanese, FR denotes french and EN denotes english.}
\begin{adjustbox}{max width=\textwidth}
\begin{tabular}{llccccc|c}
\toprule
\textbf{Datasets} &   \textbf{Language}    & \textbf{Entities} & \textbf{Rel.} & \textbf{Attr.} & \textbf{Rel. triples} & \textbf{Attr. Triples} & \textbf{Align.}\\
\midrule
% \multicolumn{7}{c}{\textbf{DBP15K}} \\
% \midrule
\multirow{2}{*}{DBP\textsubscript{ZH-EN}} & ZH & 19,388 & 1,701 & 7,780 & 70,414 & 379,684 & \multirow{2}{*}{15,000} \\
                       & EN & 19,572 & 1,323 & 6,933 & 95,142 & 567,755 & \\
\multirow{2}{*}{DBP\textsubscript{JA-EN}} & JA & 19,814 & 1,299 & 5,681 & 77,214 & 354,619 & \multirow{2}{*}{15,000}\\
                       & EN & 19,780 & 1,153 & 5,850 & 93,484 & 497,230 & \\
\multirow{2}{*}{DBP\textsubscript{FR-EN}} & FR & 19,661 &   903 & 4,431 & 105,998 & 528,665 & \multirow{2}{*}{15,000}\\
                       & EN & 19,993 & 1,208 & 6,161 & 115,722 & 576,543 & \\
% \midrule
% \multicolumn{7}{c}{\textbf{OpenEA}} \\
\midrule
\multirow{2}{*}{D\_W\_15K\_V1}   & DBpedia & 15,000 & 248 & 342 & 38,265 & 68,258 & \multirow{2}{*}{15,000}\\
                                 & Wikidata & 15,000 & 169 & 649 & 42,746 & 138,246 & \\
\multirow{2}{*}{D\_W\_15K\_V2}   & DBpedia & 15,000 & 167 & 175 & 73,983 & 66,813 & \multirow{2}{*}{15,000}\\
                                 & Wikidata & 15,000 & 121 & 457 & 83,365 & 175,686 & \\
% \midrule
\multirow{2}{*}{D\_W\_100K\_V1}  & DBpedia & 100,000 & 413 & 493 & 293,990 & 451,011 & \multirow{2}{*}{100,000}\\
                                 & Wikidata & 100,000 & 261 & 874 & 251,708 & 687,860 & \\
\multirow{2}{*}{D\_W\_100K\_V2}  & DBpedia & 100,000 & 287 & 379 & 294,188 & 523,062 & \multirow{2}{*}{100,000}\\
                                 & Wikidata & 100,000 & 32 & 38 & 400,518 & 749,787 & \\
                                 
% \midrule
\bottomrule
\end{tabular}
\end{adjustbox}
\label{tab:statistic_ea}
\end{table}

\begin{table}
\centering
\caption{Statistics of Knowledge Graph Alignment datasets. Mem-ST denotes memoryalpha-stexpanded, Star-SWT denotes starwars-swtor.}
\begin{adjustbox}{max width=\textwidth}
\begin{tabular}{llccccc}
\hline
\textbf{Datasets} & \textbf{Source} & \textbf{Inst.} & \textbf{Prop.} & \textbf{Class.} & \textbf{Triples.} & \textbf{Align.(Inst./class./prop.)}\\
\hline
\multirow{2}{*}{Star-SWT} & Star Wars Wiki & 145{,}033 & 700 & 269 & 8,246,033 & \multirow{2}{*}{1725/41/13}\\
                           & The Old Republic Wiki & 4{,}180 & 368 & 101 & 146,148 & \\

\multirow{2}{*}{Mem-ST} & Memory Alpha  & 45{,}828 & 325 & 181 & 2,526,928 & \multirow{2}{*}{9295/53/14}\\
                        & Star Trek Expanded Universe  & 13{,}426 & 202 & 283 & 567,386 & \\
\hline
\end{tabular}%
\end{adjustbox}
\label{tab:statistic_kga}
\end{table}
